# Supplementary material for: Optimal paths on the road network as directed polymers
Source: arXiv:1706.00489 ancillary file (2017-06-01)
Supplement: Supplementary file 1 [file SuppInfV1.pdf]

# Optimal paths on the road network as directed polymers
# Supplementary Information

A. P. Solon,[1] G. Bunin,[2] S. Chu,[1] and M. Kardar[1]
[1]*Department of Physics, Massachusetts Institute of Technology, Cambridge, MA 02139, USA*
[2]*Department of Physics, Technion, Haifa, 32000, Israel*
(Dated: June 1, 2017)

## I. OVERHANGS

We define here properly the overhang length $L_h$ displayed in Fig.3 (main text). Our algorithm returns a list of points $\{P_i\}$ along the path. For each of them we compute its coordinate $x_i$ on the axis running between the end points of the path. We then consider point as part of an overhang $x_i < x_j$ for some $j < i$. If the point falls outside the end points ($x < 0$ or $x > d$) it is also considered as part of an overhang. This definition is illustrated in the sketch below where the red portion of the path are defined as overhangs.

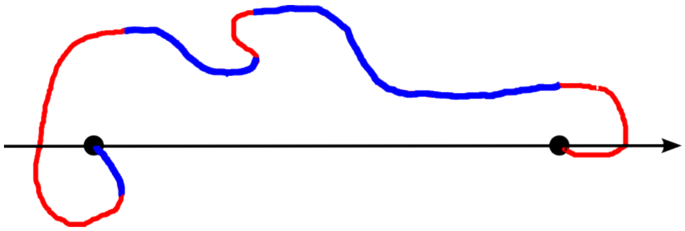

## II. CONVERGENCE OF $P(L|d)$ AND $P(T|d)$

We show in Fig. 1 the distributions $P(L|d)$ (as in Fig.5, top in main text) for the shortest paths in the US and Asia. Fig. 2 shows the equivalent curves $P(T|d)$ for the fastest paths in the three regions. Rescaling happens in a similar way as for the shortest paths except for a deviation in the Europe data set at $d = 100$km (Fig. 2 top left). In Fig. 2 (bottom, left), we plot the end points of the paths corresponding to the left bump of the distribution. They appear concentrated along the German highway network which has no speed limitations on large portions and thus allows for faster routes.

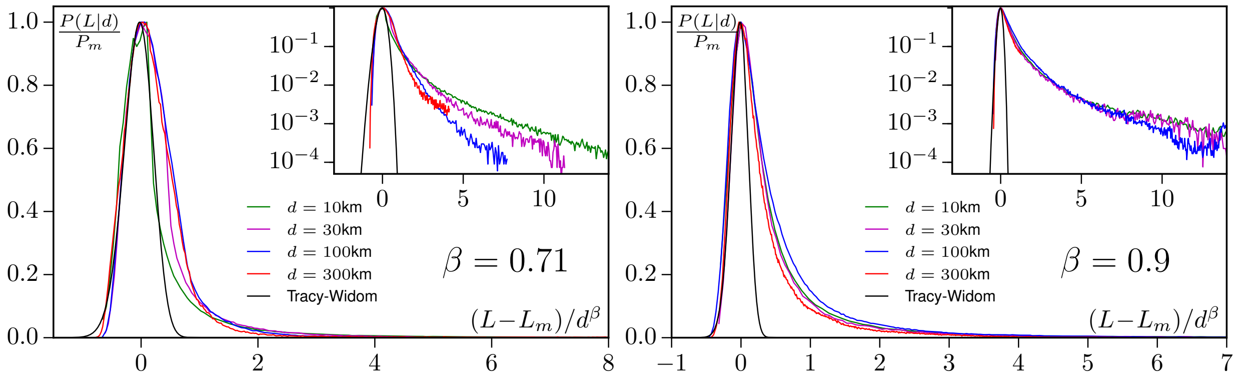


FIG. 1. Distribution of the length of the shortest path in the US (left) and Asia (right) as in Fig.5 top in main text.

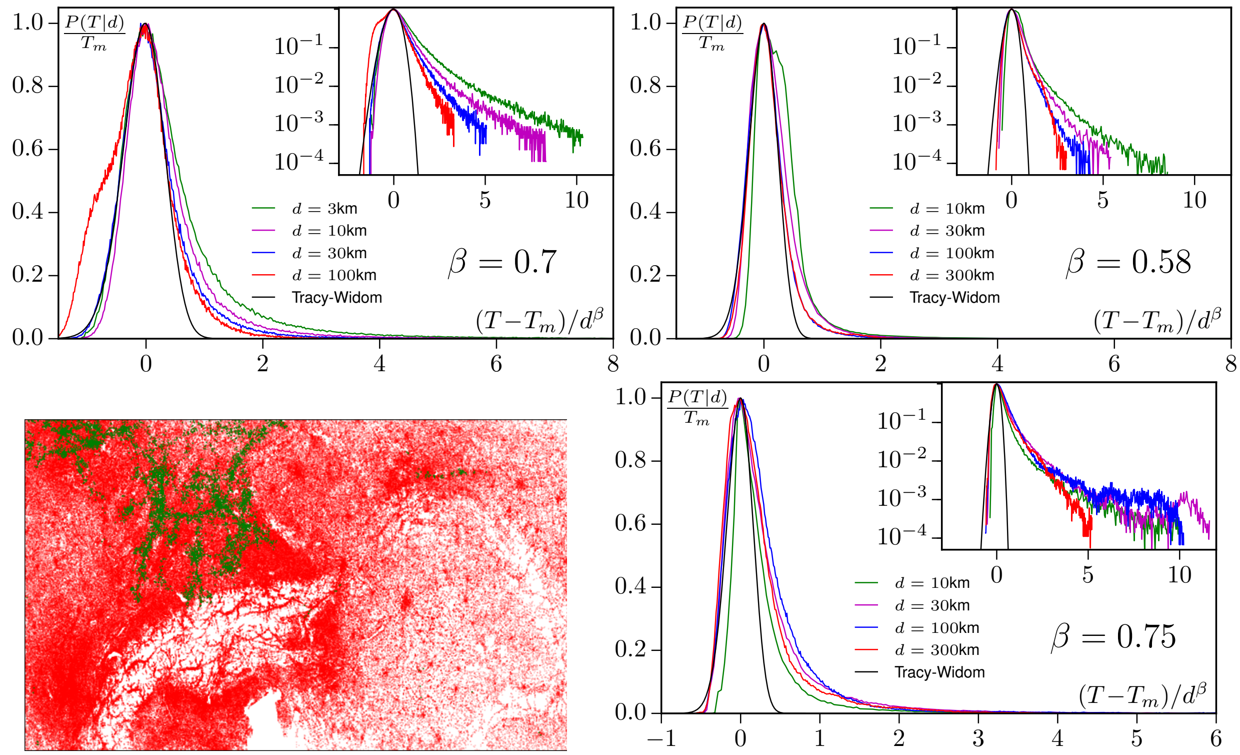


FIG. 2. Distribution of the travel time $P(T|d)$ on the fastest paths in Europe (top left), the US (top right) and Asia (bottom right). The bottom left corner shows the end points of the paths between points at distance $d = 100$km sampled in the top left figure. Green points correspond to the fast paths $T < 4500$ that make up the left bump in the distribution. Red points correspond to all slower paths.
